# Supplementary material for: Accurate Excitation Energies of Point Defects from Fast Particle-Particle Random Approximation Calculations
Source: arXiv:2401.10483 ancillary file (2024-01-19)
Supplement: Supplementary file 1 [file supporting_information.pdf]

**Supporting Information:**

**Accurate Excitation Energies of Point Defects**

**from Fast Particle-Particle Random**

**Approximation Calculations**

Jiachen Li,<sup>\*,†</sup> Yu Jin,<sup>‡</sup> Jincheng Yu,<sup>¶</sup> Weitao Yang,<sup>\*,¶</sup> and Tianyu Zhu<sup>\*,†</sup>

*<sup>†</sup>Department of Chemistry, Yale University, New Haven, CT, USA 06520*

*<sup>‡</sup>Department of Chemistry, University of Chicago, Chicago, Illinois 60637, United States*

*<sup>¶</sup>Department of Chemistry, Duke University, Durham, NC 27708, USA*

E-mail: jiachen.li@yale.edu; weitao.yang@duke.edu; tianyu.zhu@yale.edu

# 1 Details about geometry optimizations

We obtained the ground-state equilibrium atomic geometries of point defects in diamond and 4H-SiC using density functional theory<sup>S1,S2</sup> (DFT) and the plane-wave pseudopotential method, as implemented in the Quantum ESPRESSO package,<sup>S3,S4</sup> by minimizing the nuclear forces below the threshold of 0.01 eV Å<sup>-1</sup>. Our study involved unrestricted Kohn-Sham DFT calculations for the triplet ground states, specifically the <sup>3</sup>A<sub>2</sub> ground state of NV<sup>-</sup> in diamond, *kk*-VV<sup>0</sup> in 4H-SiC, and the <sup>3</sup>A<sub>2g</sub> ground state of SiV<sup>0</sup> in diamond. We used SG15 ONCV norm-conserving pseudopotentials<sup>S5,S6</sup> and the PBE<sup>S7</sup> functional with the plane-wave energy cutoff setting to 60 Ry.

# 2 Excitation energies of defects obtained from ppRPA

Table S1: Vertical excitation energies of NV<sup>-</sup> in diamond obtained from ppRPA@PBE and ppRPA@B3LYP with the supercell model containing 63 atoms. (*O*, *V*) means that *O* occupied orbitals and *V* virtual orbitals were used in the active space. The geometry of the <sup>3</sup>A<sub>2</sub> ground state and cc-pVDZ basis set were used. All values are in eV.

|         | ppRPA@PBE      |                             |                | ppRPA@B3LYP    |                             |                |
|---------|----------------|-----------------------------|----------------|----------------|-----------------------------|----------------|
|         | <sup>1</sup> E | <sup>1</sup> A <sub>1</sub> | <sup>3</sup> E | <sup>1</sup> E | <sup>1</sup> A <sub>1</sub> | <sup>3</sup> E |
| (10,10) | 0.56           | 1.75                        | 1.88           | 0.63           | 1.98                        | 2.08           |
| (20,20) | 0.56           | 1.74                        | 1.89           | 0.62           | 1.98                        | 2.09           |
| (30,30) | 0.55           | 1.68                        | 1.89           | 0.61           | 1.92                        | 2.09           |
| (40,40) | 0.54           | 1.68                        | 1.86           | 0.61           | 1.91                        | 2.07           |
| (50,50) | 0.54           | 1.65                        | 1.86           | 0.60           | 1.88                        | 2.07           |
| (60,60) | 0.53           | 1.63                        | 1.86           | 0.60           | 1.86                        | 2.07           |
| (70,70) | 0.53           | 1.63                        | 1.86           | 0.60           | 1.86                        | 2.07           |
| (80,80) | 0.53           | 1.63                        | 1.86           | 0.60           | 1.86                        | 2.07           |
| (90,90) | 0.53           | 1.62                        | 1.86           | 0.60           | 1.86                        | 2.07           |

Table S1: Continued

|           | ppRPA@PBE      |                             |                | ppRPA@B3LYP    |                             |                |
|-----------|----------------|-----------------------------|----------------|----------------|-----------------------------|----------------|
|           | <sup>1</sup> E | <sup>1</sup> A <sub>1</sub> | <sup>3</sup> E | <sup>1</sup> E | <sup>1</sup> A <sub>1</sub> | <sup>3</sup> E |
| (100,100) | 0.53           | 1.62                        | 1.86           | 0.59           | 1.85                        | 2.07           |
| (110,110) | 0.53           | 1.60                        | 1.86           | 0.59           | 1.84                        | 2.07           |
| (120,120) | 0.52           | 1.59                        | 1.86           | 0.59           | 1.83                        | 2.07           |
| (130,130) | 0.52           | 1.59                        | 1.86           | 0.59           | 1.82                        | 2.07           |
| (140,140) | 0.52           | 1.59                        | 1.86           | 0.59           | 1.82                        | 2.07           |
| (150,150) | 0.52           | 1.59                        | 1.86           | 0.59           | 1.82                        | 2.07           |
| (160,160) | 0.52           | 1.58                        | 1.86           | 0.59           | 1.82                        | 2.07           |
| (170,170) | 0.52           | 1.58                        | 1.86           | 0.59           | 1.82                        | 2.07           |
| (180,180) | 0.52           | 1.58                        | 1.87           | 0.59           | 1.82                        | 2.07           |
| (190,190) | 0.52           | 1.57                        | 1.87           | 0.58           | 1.81                        | 2.07           |
| (191,200) | 0.52           | 1.57                        | 1.87           | 0.58           | 1.81                        | 2.07           |

Table S2: Vertical excitation energies of NV<sup>-</sup> in diamond obtained from ppRPA@PBE and ppRPA@B3LYP with the supercell model containing 215 atoms. (*O*, *V*) means that *O* occupied orbitals and *V* virtual orbitals were used in the active space. The geometry of the <sup>3</sup>A<sub>2</sub> ground state and cc-pVDZ basis set were used. All values are in eV.

|         | ppRPA@PBE      |                             |                | ppRPA@B3LYP    |                             |                |
|---------|----------------|-----------------------------|----------------|----------------|-----------------------------|----------------|
|         | <sup>1</sup> E | <sup>1</sup> A <sub>1</sub> | <sup>3</sup> E | <sup>1</sup> E | <sup>1</sup> A <sub>1</sub> | <sup>3</sup> E |
| (10,10) | 0.57           | 1.80                        | 1.97           | 0.64           | 2.08                        | 2.13           |
| (20,20) | 0.55           | 1.74                        | 1.96           | 0.63           | 2.02                        | 2.12           |
| (30,30) | 0.55           | 1.73                        | 1.94           | 0.62           | 2.00                        | 2.10           |
| (40,40) | 0.55           | 1.72                        | 1.93           | 0.62           | 2.00                        | 2.10           |
| (50,50) | 0.54           | 1.70                        | 1.93           | 0.62           | 1.98                        | 2.10           |

Table S2: Continued

|           | ppRPA@PBE |         |       | ppRPA@B3LYP |         |       |
|-----------|-----------|---------|-------|-------------|---------|-------|
|           | $^1E$     | $^1A_1$ | $^3E$ | $^1E$       | $^1A_1$ | $^3E$ |
| (60,60)   | 0.54      | 1.69    | 1.93  | 0.61        | 1.97    | 2.10  |
| (70,70)   | 0.54      | 1.69    | 1.93  | 0.61        | 1.97    | 2.10  |
| (80,80)   | 0.54      | 1.68    | 1.93  | 0.61        | 1.96    | 2.10  |
| (90,90)   | 0.53      | 1.68    | 1.93  | 0.61        | 1.95    | 2.09  |
| (100,100) | 0.53      | 1.67    | 1.93  | 0.61        | 1.95    | 2.09  |
| (110,110) | 0.53      | 1.67    | 1.93  | 0.61        | 1.95    | 2.09  |
| (120,120) | 0.53      | 1.67    | 1.93  | 0.61        | 1.94    | 2.09  |
| (130,130) | 0.53      | 1.66    | 1.93  | 0.61        | 1.94    | 2.09  |
| (140,140) | 0.53      | 1.66    | 1.93  | 0.61        | 1.94    | 2.09  |
| (150,150) | 0.53      | 1.66    | 1.93  | 0.61        | 1.94    | 2.09  |
| (160,160) | 0.53      | 1.66    | 1.93  | 0.61        | 1.94    | 2.09  |
| (170,170) | 0.53      | 1.66    | 1.93  | 0.60        | 1.94    | 2.09  |
| (180,180) | 0.53      | 1.64    | 1.93  | 0.60        | 1.93    | 2.09  |
| (190,190) | 0.52      | 1.64    | 1.93  | 0.60        | 1.92    | 2.09  |
| (200,200) | 0.52      | 1.64    | 1.92  | 0.60        | 1.92    | 2.09  |

Table S3: Vertical excitation energies of  $SiV^0$  in diamond obtained from ppRPA@PBE and ppRPA@B3LYP with the supercell model containing 63 atoms. ( $O$ ,  $V$ ) means that  $O$  occupied orbitals and  $V$  virtual orbitals were used in the active space. The geometry of the  $^3A_{2g}$  ground state and cc-pVDZ basis set were used. All values are in eV.

|         | ppRPA@PBE  |         |            | ppRPA@B3LYP |         |            |
|---------|------------|---------|------------|-------------|---------|------------|
|         | $^3A_{2u}$ | $^3E_u$ | $^3A_{1u}$ | $^3A_{2u}$  | $^3E_u$ | $^3A_{1u}$ |
| (10,10) | 1.92       | 2.09    | 2.58       | 2.00        | 2.18    | 2.62       |

Table S3: Continued

|           | ppRPA@PBE  |         |            | ppRPA@B3LYP |         |            |
|-----------|------------|---------|------------|-------------|---------|------------|
|           | $^3A_{2u}$ | $^3E_u$ | $^3A_{1u}$ | $^3A_{2u}$  | $^3E_u$ | $^3A_{1u}$ |
| (20,20)   | 1.92       | 2.09    | 2.57       | 2.01        | 2.18    | 2.66       |
| (30,30)   | 1.94       | 2.11    | 2.54       | 2.03        | 2.20    | 2.63       |
| (40,40)   | 1.97       | 2.12    | 2.51       | 2.05        | 2.21    | 2.61       |
| (50,50)   | 1.94       | 2.10    | 2.48       | 2.03        | 2.20    | 2.58       |
| (60,60)   | 1.94       | 2.11    | 2.47       | 2.03        | 2.20    | 2.57       |
| (70,70)   | 1.94       | 2.10    | 2.47       | 2.03        | 2.20    | 2.56       |
| (80,80)   | 1.94       | 2.11    | 2.47       | 2.03        | 2.20    | 2.56       |
| (90,90)   | 1.94       | 2.11    | 2.46       | 2.03        | 2.20    | 2.56       |
| (100,100) | 1.94       | 2.11    | 2.46       | 2.03        | 2.20    | 2.56       |
| (110,110) | 1.94       | 2.11    | 2.46       | 2.03        | 2.20    | 2.56       |
| (120,120) | 1.94       | 2.11    | 2.46       | 2.03        | 2.20    | 2.55       |
| (130,130) | 1.94       | 2.11    | 2.46       | 2.03        | 2.20    | 2.55       |
| (140,140) | 1.94       | 2.11    | 2.46       | 2.03        | 2.20    | 2.55       |
| (150,150) | 1.95       | 2.11    | 2.46       | 2.03        | 2.20    | 2.55       |
| (160,160) | 1.95       | 2.11    | 2.46       | 2.03        | 2.20    | 2.55       |
| (170,170) | 1.95       | 2.11    | 2.46       | 2.03        | 2.20    | 2.55       |
| (180,180) | 1.95       | 2.11    | 2.46       | 2.03        | 2.20    | 2.55       |
| (190,190) | 1.95       | 2.11    | 2.46       | 2.03        | 2.20    | 2.55       |
| (194,200) | 1.95       | 2.11    | 2.46       | 2.03        | 2.20    | 2.55       |

Table S4: Vertical excitation energies of  $\text{SiV}^0$  in diamond obtained from ppRPA@PBE and ppRPA@B3LYP with the supercell model containing 215 atoms. ( $O$ ,  $V$ ) means that  $O$  occupied orbitals and  $V$  virtual orbitals were used in the active space. The geometry of the  ${}^3\text{A}_{2g}$  ground state and cc-pVDZ basis set were used. All values are in eV.

|           | ppRPA@PBE           |                  |                     | ppRPA@B3LYP         |                  |                     |
|-----------|---------------------|------------------|---------------------|---------------------|------------------|---------------------|
|           | ${}^3\text{A}_{2u}$ | ${}^3\text{E}_u$ | ${}^3\text{A}_{1u}$ | ${}^3\text{A}_{2u}$ | ${}^3\text{E}_u$ | ${}^3\text{A}_{1u}$ |
| (10,10)   | 1.52                | 1.64             | 2.08                | 1.59                | 1.71             | 2.17                |
| (20,20)   | 1.52                | 1.58             | 2.00                | 1.59                | 1.66             | 2.09                |
| (30,30)   | 1.51                | 1.57             | 1.90                | 1.57                | 1.64             | 1.96                |
| (40,40)   | 1.51                | 1.57             | 1.85                | 1.58                | 1.65             | 1.94                |
| (50,50)   | 1.50                | 1.58             | 1.84                | 1.57                | 1.65             | 1.93                |
| (60,60)   | 1.49                | 1.56             | 1.83                | 1.55                | 1.63             | 1.92                |
| (70,70)   | 1.47                | 1.54             | 1.83                | 1.54                | 1.62             | 1.91                |
| (80,80)   | 1.47                | 1.54             | 1.82                | 1.54                | 1.62             | 1.91                |
| (90,90)   | 1.47                | 1.54             | 1.82                | 1.54                | 1.62             | 1.90                |
| (100,100) | 1.47                | 1.54             | 1.81                | 1.54                | 1.62             | 1.90                |
| (110,110) | 1.47                | 1.54             | 1.81                | 1.54                | 1.62             | 1.90                |
| (120,120) | 1.47                | 1.54             | 1.81                | 1.54                | 1.61             | 1.90                |
| (130,130) | 1.47                | 1.54             | 1.81                | 1.54                | 1.61             | 1.90                |
| (140,140) | 1.47                | 1.54             | 1.81                | 1.54                | 1.61             | 1.90                |
| (150,150) | 1.47                | 1.54             | 1.81                | 1.54                | 1.61             | 1.90                |
| (160,160) | 1.47                | 1.54             | 1.81                | 1.54                | 1.62             | 1.90                |
| (170,170) | 1.47                | 1.54             | 1.81                | 1.54                | 1.62             | 1.90                |
| (180,180) | 1.47                | 1.54             | 1.81                | 1.54                | 1.62             | 1.90                |
| (190,190) | 1.47                | 1.54             | 1.81                | 1.54                | 1.62             | 1.90                |
| (200,200) | 1.47                | 1.54             | 1.81                | 1.54                | 1.62             | 1.89                |

Table S5: Vertical excitation energies of  $kk$ -VV<sup>0</sup> in 4H-SiC obtained from ppRPA@PBE and ppRPA@B3LYP with the supercell model containing 215 atoms. ( $O$ ,  $V$ ) means that  $O$  occupied orbitals and  $V$  virtual orbitals were used in the active space. The geometry of the <sup>3</sup>A<sub>2</sub> ground state and cc-pVDZ basis set were used. All values are in eV.

|           | ppRPA@PBE      |                             |                | ppRPA@B3LYP    |                             |                |
|-----------|----------------|-----------------------------|----------------|----------------|-----------------------------|----------------|
|           | <sup>1</sup> E | <sup>1</sup> A <sub>1</sub> | <sup>3</sup> E | <sup>1</sup> E | <sup>1</sup> A <sub>1</sub> | <sup>3</sup> E |
| (10,10)   | 0.31           | 1.28                        | 1.10           | 0.36           | 1.47                        | 1.18           |
| (20,20)   | 0.29           | 0.96                        | 1.15           | 0.35           | 1.13                        | 1.17           |
| (30,30)   | 0.28           | 0.90                        | 1.14           | 0.35           | 1.18                        | 1.30           |
| (40,40)   | 0.29           | 0.89                        | 1.16           | 0.35           | 1.15                        | 1.27           |
| (50,50)   | 0.28           | 0.88                        | 1.13           | 0.34           | 1.13                        | 1.27           |
| (60,60)   | 0.29           | 0.88                        | 1.12           | 0.34           | 1.15                        | 1.24           |
| (70,70)   | 0.28           | 0.88                        | 1.14           | 0.34           | 1.14                        | 1.23           |
| (80,80)   | 0.28           | 0.87                        | 1.12           | 0.34           | 1.13                        | 1.23           |
| (90,90)   | 0.28           | 0.87                        | 1.12           | 0.34           | 1.13                        | 1.24           |
| (100,100) | 0.28           | 0.87                        | 1.12           | 0.34           | 1.13                        | 1.24           |
| (110,110) | 0.28           | 0.87                        | 1.12           | 0.34           | 1.13                        | 1.24           |
| (120,120) | 0.28           | 0.87                        | 1.12           | 0.33           | 1.13                        | 1.23           |
| (130,130) | 0.28           | 0.87                        | 1.12           | 0.33           | 1.13                        | 1.24           |
| (140,140) | 0.28           | 0.87                        | 1.12           | 0.33           | 1.13                        | 1.24           |
| (150,150) | 0.28           | 0.87                        | 1.12           | 0.33           | 1.13                        | 1.24           |
| (160,160) | 0.28           | 0.87                        | 1.12           | 0.33           | 1.13                        | 1.24           |
| (170,170) | 0.28           | 0.87                        | 1.12           | 0.33           | 1.13                        | 1.24           |
| (180,180) | 0.28           | 0.87                        | 1.12           | 0.33           | 1.13                        | 1.24           |
| (190,190) | 0.28           | 0.87                        | 1.12           | 0.33           | 1.13                        | 1.24           |
| (200,200) | 0.28           | 0.88                        | 1.12           | 0.33           | 1.13                        | 1.23           |

### 3 Basis set convergence

Vertical excitation energies of  $\text{NV}^-$  in diamond obtained from ppRPA@PBE and ppRPA@B3LYP with the cc-pVTZ basis set<sup>S8</sup> and the supercell model containing 63 atoms are tabulated in Table.S6. It shows that excitation energies obtained from ppRPA with the cc-pVTZ basis set are very similar to those with the cc-pVDZ basis set in Table.S1. Thus, we used cc-pVDZ basis set for ppRPA calculations in this work.

Table S6: Vertical excitation energies of  $\text{NV}^-$  in diamond obtained from ppRPA@PBE and ppRPA@B3LYP with cc-pVTZ basis set. ( $O$ ,  $V$ ) means that  $O$  occupied orbitals and  $V$  virtual orbitals were used in the active space. The geometry of the  $^3\text{A}_2$  ground state and the supercell model containing 63 atoms were used. All values are in eV.

|           | ppRPA@PBE    |                |              | ppRPA@B3LYP  |                |              |
|-----------|--------------|----------------|--------------|--------------|----------------|--------------|
|           | $^1\text{E}$ | $^1\text{A}_1$ | $^3\text{E}$ | $^1\text{E}$ | $^1\text{A}_1$ | $^3\text{E}$ |
| (10,10)   | 0.56         | 1.74           | 1.87         | 0.63         | 1.98           | 2.08         |
| (20,20)   | 0.56         | 1.74           | 1.88         | 0.63         | 1.97           | 2.08         |
| (30,30)   | 0.55         | 1.68           | 1.88         | 0.61         | 1.91           | 2.08         |
| (40,40)   | 0.55         | 1.68           | 1.86         | 0.61         | 1.91           | 2.07         |
| (50,50)   | 0.54         | 1.65           | 1.86         | 0.60         | 1.88           | 2.07         |
| (60,60)   | 0.53         | 1.63           | 1.86         | 0.60         | 1.86           | 2.06         |
| (70,70)   | 0.53         | 1.63           | 1.86         | 0.60         | 1.86           | 2.06         |
| (80,80)   | 0.53         | 1.62           | 1.86         | 0.60         | 1.86           | 2.06         |
| (90,90)   | 0.53         | 1.62           | 1.86         | 0.59         | 1.85           | 2.06         |
| (100,100) | 0.53         | 1.62           | 1.86         | 0.59         | 1.85           | 2.06         |
| (110,110) | 0.53         | 1.60           | 1.86         | 0.59         | 1.83           | 2.06         |
| (120,120) | 0.52         | 1.59           | 1.86         | 0.59         | 1.83           | 2.06         |
| (130,130) | 0.52         | 1.59           | 1.86         | 0.59         | 1.82           | 2.06         |
| (140,140) | 0.52         | 1.58           | 1.86         | 0.59         | 1.82           | 2.06         |

Table S6: Continued

|           | ppRPA@PBE      |                             |                | ppRPA@B3LYP    |                             |                |
|-----------|----------------|-----------------------------|----------------|----------------|-----------------------------|----------------|
|           | <sup>1</sup> E | <sup>1</sup> A <sub>1</sub> | <sup>3</sup> E | <sup>1</sup> E | <sup>1</sup> A <sub>1</sub> | <sup>3</sup> E |
| (150,150) | 0.52           | 1.58                        | 1.86           | 0.59           | 1.82                        | 2.06           |
| (160,160) | 0.52           | 1.58                        | 1.86           | 0.59           | 1.82                        | 2.06           |
| (170,170) | 0.52           | 1.58                        | 1.86           | 0.59           | 1.82                        | 2.06           |
| (180,180) | 0.52           | 1.57                        | 1.86           | 0.58           | 1.81                        | 2.06           |
| (190,190) | 0.52           | 1.57                        | 1.86           | 0.58           | 1.81                        | 2.06           |
| (200,200) | 0.52           | 1.57                        | 1.86           | 0.58           | 1.80                        | 2.06           |

## References

- (S1) Hohenberg, P.; Kohn, W. Inhomogeneous Electron Gas. *Phys. Rev.* **1964**, *136*, B864–B871.
- (S2) Parr, R. G.; Weitao, Y. *Density-Functional Theory of Atoms and Molecules*; Oxford University Press, 1989.
- (S3) Giannozzi, P.; Barone, O.; Bonfà, P.; Brunato, D.; Car, R.; Carnimeo, I.; Cavazzoni, C.; de Gironcoli, S.; Delugas, P.; Ferrari Ruffino, F.; Ferretti, A.; Marzari, N.; Timrov, I.; Urru, A.; Baroni, S. Quantum ESPRESSO toward the Exascale. *J. Chem. Phys.* **2020**, *152*, 154105.
- (S4) Carnimeo, I.; Affinito, F.; Baroni, S.; Barone, O.; Bellentani, L.; Bertossa, R.; Delugas, P. D.; Ruffino, F. F.; Orlandini, S.; Spiga, F.; Giannozzi, P. Quantum ESPRESSO: One Further Step toward the Exascale. *J. Chem. Theory Comput.* **2023**, *19*, 6992–7006.

- (S5) Hamann, D. R. Optimized Norm-Conserving Vanderbilt Pseudopotentials. *Phys. Rev. B* **2013**, *88*, 085117.
- (S6) Schlipf, M.; Gygi, F. Optimization Algorithm for the Generation of ONCV Pseudopotentials. *Computer Physics Communications* **2015**, *196*, 36–44.
- (S7) Perdew, J. P.; Burke, K.; Ernzerhof, M. Generalized Gradient Approximation Made Simple. *Phys. Rev. Lett.* **1996**, *77*, 3865–3868.
- (S8) Dunning, T. H. Gaussian Basis Sets for Use in Correlated Molecular Calculations. I. The Atoms Boron through Neon and Hydrogen. *J. Chem. Phys.* **1989**, *90*, 1007–1023.
